# Supplementary material for: Adaptive and Robust Watermark for Generative Tabular Data
Source: arXiv:2409.14700 source file (2026-07-08)
Supplement: Supplementary file 1 [file appendix-on-categorical-data.tex]

\section{Watermarking for categorical data}

We begin by stating the algorithm for watermaking data in the pre-generation phase. 

\begin{algorithm}[H]
    \caption{Pre-generation min-hash watermarking -- pseudocode}
    \label{alg:pre-generation-min-hash-encoding}
    \begin{algorithmic}[1]
        \REQUIRE Seed cells of a row $\{\bv c_1, \ldots, \bv c_k\}$, number of cells to generate $t \in \mathbb{N}^+$, generator algorithm $\mathcal{A}: \R^{k\times m} \to \R^{t\times d}$, two large prime numbers $p_1, p_2 \in \mathbb{N}^+$, random projection function $\pi: \R^d \to \R^q$, and partition function $f: \R^q \to \{R, G\}$, final output function $o: \R^{t\times q} \to |\mathcal{S}|^t$, where $|S|$ is the set of values corresponding to each columns. \ray{one can imagine $o$ mapping to independent sets $\{\mathcal{S}_1, \ldots, \mathcal{S}_t\}$.}
        \STATE Compute $\bv M = \mathcal{A}(\{\bv c_1, \ldots, \bv c_k\})$.
        \STATE Compute $\bar{\bv M} = \pi(\bv M)$, where $\pi$ is initialized with the seed $p_1$. \ray{this can be replaced with a subspace splitting algorithm, but I am not sure how to use LSH kind of algorithms to do that implicitly.}
        \STATE Compute random features $\bv F$ in $\R^q$ using the seed $p_2$.
        \STATE Project $\bar{\bv M}$ on the column space of $\bv F$ to get $\bv E \in \R^{t\times q}$.
        \STATE Run function $o$ on each row of $t$ to generate the corresponding cell in the row.
        \STATE \ray{\textbf{comment}: one can imagine doing this sequentially, but that would not allow verification in case of column subsamples. This is a sketch algorithm, and may contain bugs in the dimensions of the functions I am constructing.}
    \end{algorithmic}
\end{algorithm}

\paragraph{Runtime.} \ray{TODO}

\paragraph{Overview of the algorithm.} Given prime $p_1$ we construct the random projection of the vectors generated by $\mathcal{A}$ immediately before it maps to the set of values. We then use $p_2$ to draw random Fourier features in the same space. Then these embeddings are mapped to space spanned by these random fourier features (ensuring the columns are spanned by the features we drew "randomly" using a fixed seed). The output function basically runs on these vectors to generate the table. \ray{we need to show that create a uniquely identifiable partition when the embedding space is actually the output space the adversarial query generation becomes increasing simpler.}

\subsection{Proof requirements}
\begin{itemize}
    \item We show that the above function can be uniquely identified by satisfying the hypothesis test: 
    \begin{center}
        \emph{$H_0$: The text is not generated knowing a rule of valid blocked partitions of the semantic space.}
    \end{center}
    See \cite{hou2023semstamp} for a direction of how to do this.

    \item We show that the resultant tabular data is close in the Wasserstein distance when the generator algorithm $\mathcal{A}: S \to \R^d$.
    \item We show that when the generator algorithm $\mathcal{A}: S \to \{0,1\}^d$, then the Wasserstein distance to ensure watermark is detectable is too large. Conversely, we show that if Wasserstein distance is small, then the detection algorithm has to be exponential time, to avoid watermarking being broken by an adversary in polynomial time.
    \item We finally show that as $|T| \to \infty$ for a generator algorithm $\mathcal{A}: S \to T^d$, the Wasserstein distance can be small and the watermark detection algorithm can run in polynomial time.
    \item Show as long as seed cells are maintained, we can always verify each row even when presented with a subsample.
\end{itemize}
