# Supplementary material for: Adaptive and Robust Watermark for Generative Tabular Data
Source: arXiv:2409.14700 source file (2026-07-08)
Supplement: Supplementary file 2 [file appendix-details-experiments.tex]

\section{Settings of Experiments}

\label{appendix:experiment-details}
For synthetic data generation using three generative methods mentioned in the paper, we follow  the default hyperparameters found in the SDV library ~\cite{patki2016synthetic}. We run the experiments on a machine type of g4dn.4xlarge consisting of 16 CPU, 64GB RAM, and 1 GPU. For Utility evaluation, default parameters of the XGBoost classifier ~\cite{chen2016xgboost} and Random Forest classifier with a seed of 42 was used. The synthetic data generation, training and evaluation process typically finishes within 4 hrs. Python 3.8 version was used to run the experiments.
